# Supplementary material for: The eta-local motivic sphere
Source: arXiv:1406.7733 ancillary file (2014-06-30)

ABSTRACT. This document contains large-format charts of the  $h_1$ -localized motivic May spectral sequence that computes the  $h_1$ -localized cohomology of the motivic Steenrod algebra over  $\mathbb{C}$ . The charts are complete through the Milnor-Witt 66-stem.

This document contains large-format charts of the  $h_1$ -localized motivic May spectral sequence that computes the  $h_1$ -localized cohomology of the motivic Steenrod algebra over  $\mathbb{C}$ . The charts are complete through the Milnor-Witt 66-stem.

These charts are a companion to [1], which explains the notation and justifies the calculations.

The charts are formatted for paper measuring 34 inches by 22 inches, which is approximately equivalent to A1 paper.

The following is a key for reading the charts.

- (1) The horizontal axes indicate the Milnor-Witt stem, i.e., the stem minus the motivic weight.
- (2) The vertical axes indicate the May filtration minus the Adams filtration.
- (3) Dots indicate copies of  $\mathbb{F}_2$ .
- (4) All of our calculations are free as a module over the polynomial ring  $\mathbb{F}_2[P]$ , so the charts only show the spectral sequence modulo  $P$ . The solid squares labelled  $P$  serve as a reminder of this.
- (5) Lines of slope  $2/3$  indicate multiplications by  $c_0$ .
- (6) Arrows of slope  $2/3$  indicate infinitely many multiplications by  $c_0$ .
- (7) Horizontal blue lines indicate multiplications by  $h_4$ .
- (8) The May  $d_r$  differential takes elements one unit to the left and  $r$  units downward.

In addition to the May  $d_{16}$  differentials, the chart of the  $E_{16}$ -page also indicates the remaining higher differentials. In our range, all differentials except for  $d_{18}$  and  $d_{32}$  are trivial.

#### REFERENCES

- [1] B. J. Guillou and D. C. Isaksen, *The  $\eta$ -local motivic sphere*, 2014, preprint.

2000 *Mathematics Subject Classification*. 55T15, 55S10, 14F42.

*Key words and phrases*. cohomology of the Steenrod algebra, May spectral sequence, motivic stable homotopy group.

bertguillou@uky.edu

DEPARTMENT OF MATHEMATICS, UNIVERSITY OF KENTUCKY, LEXINGTON, KY 40506, USA

The first author was supported by Simons Collaboration Grant 282316.

isaksen@wayne.edu

DEPARTMENT OF MATHEMATICS, WAYNE STATE UNIVERSITY, DETROIT, MI 48202, USA

The second author was supported by NSF grant DMS-1202213.

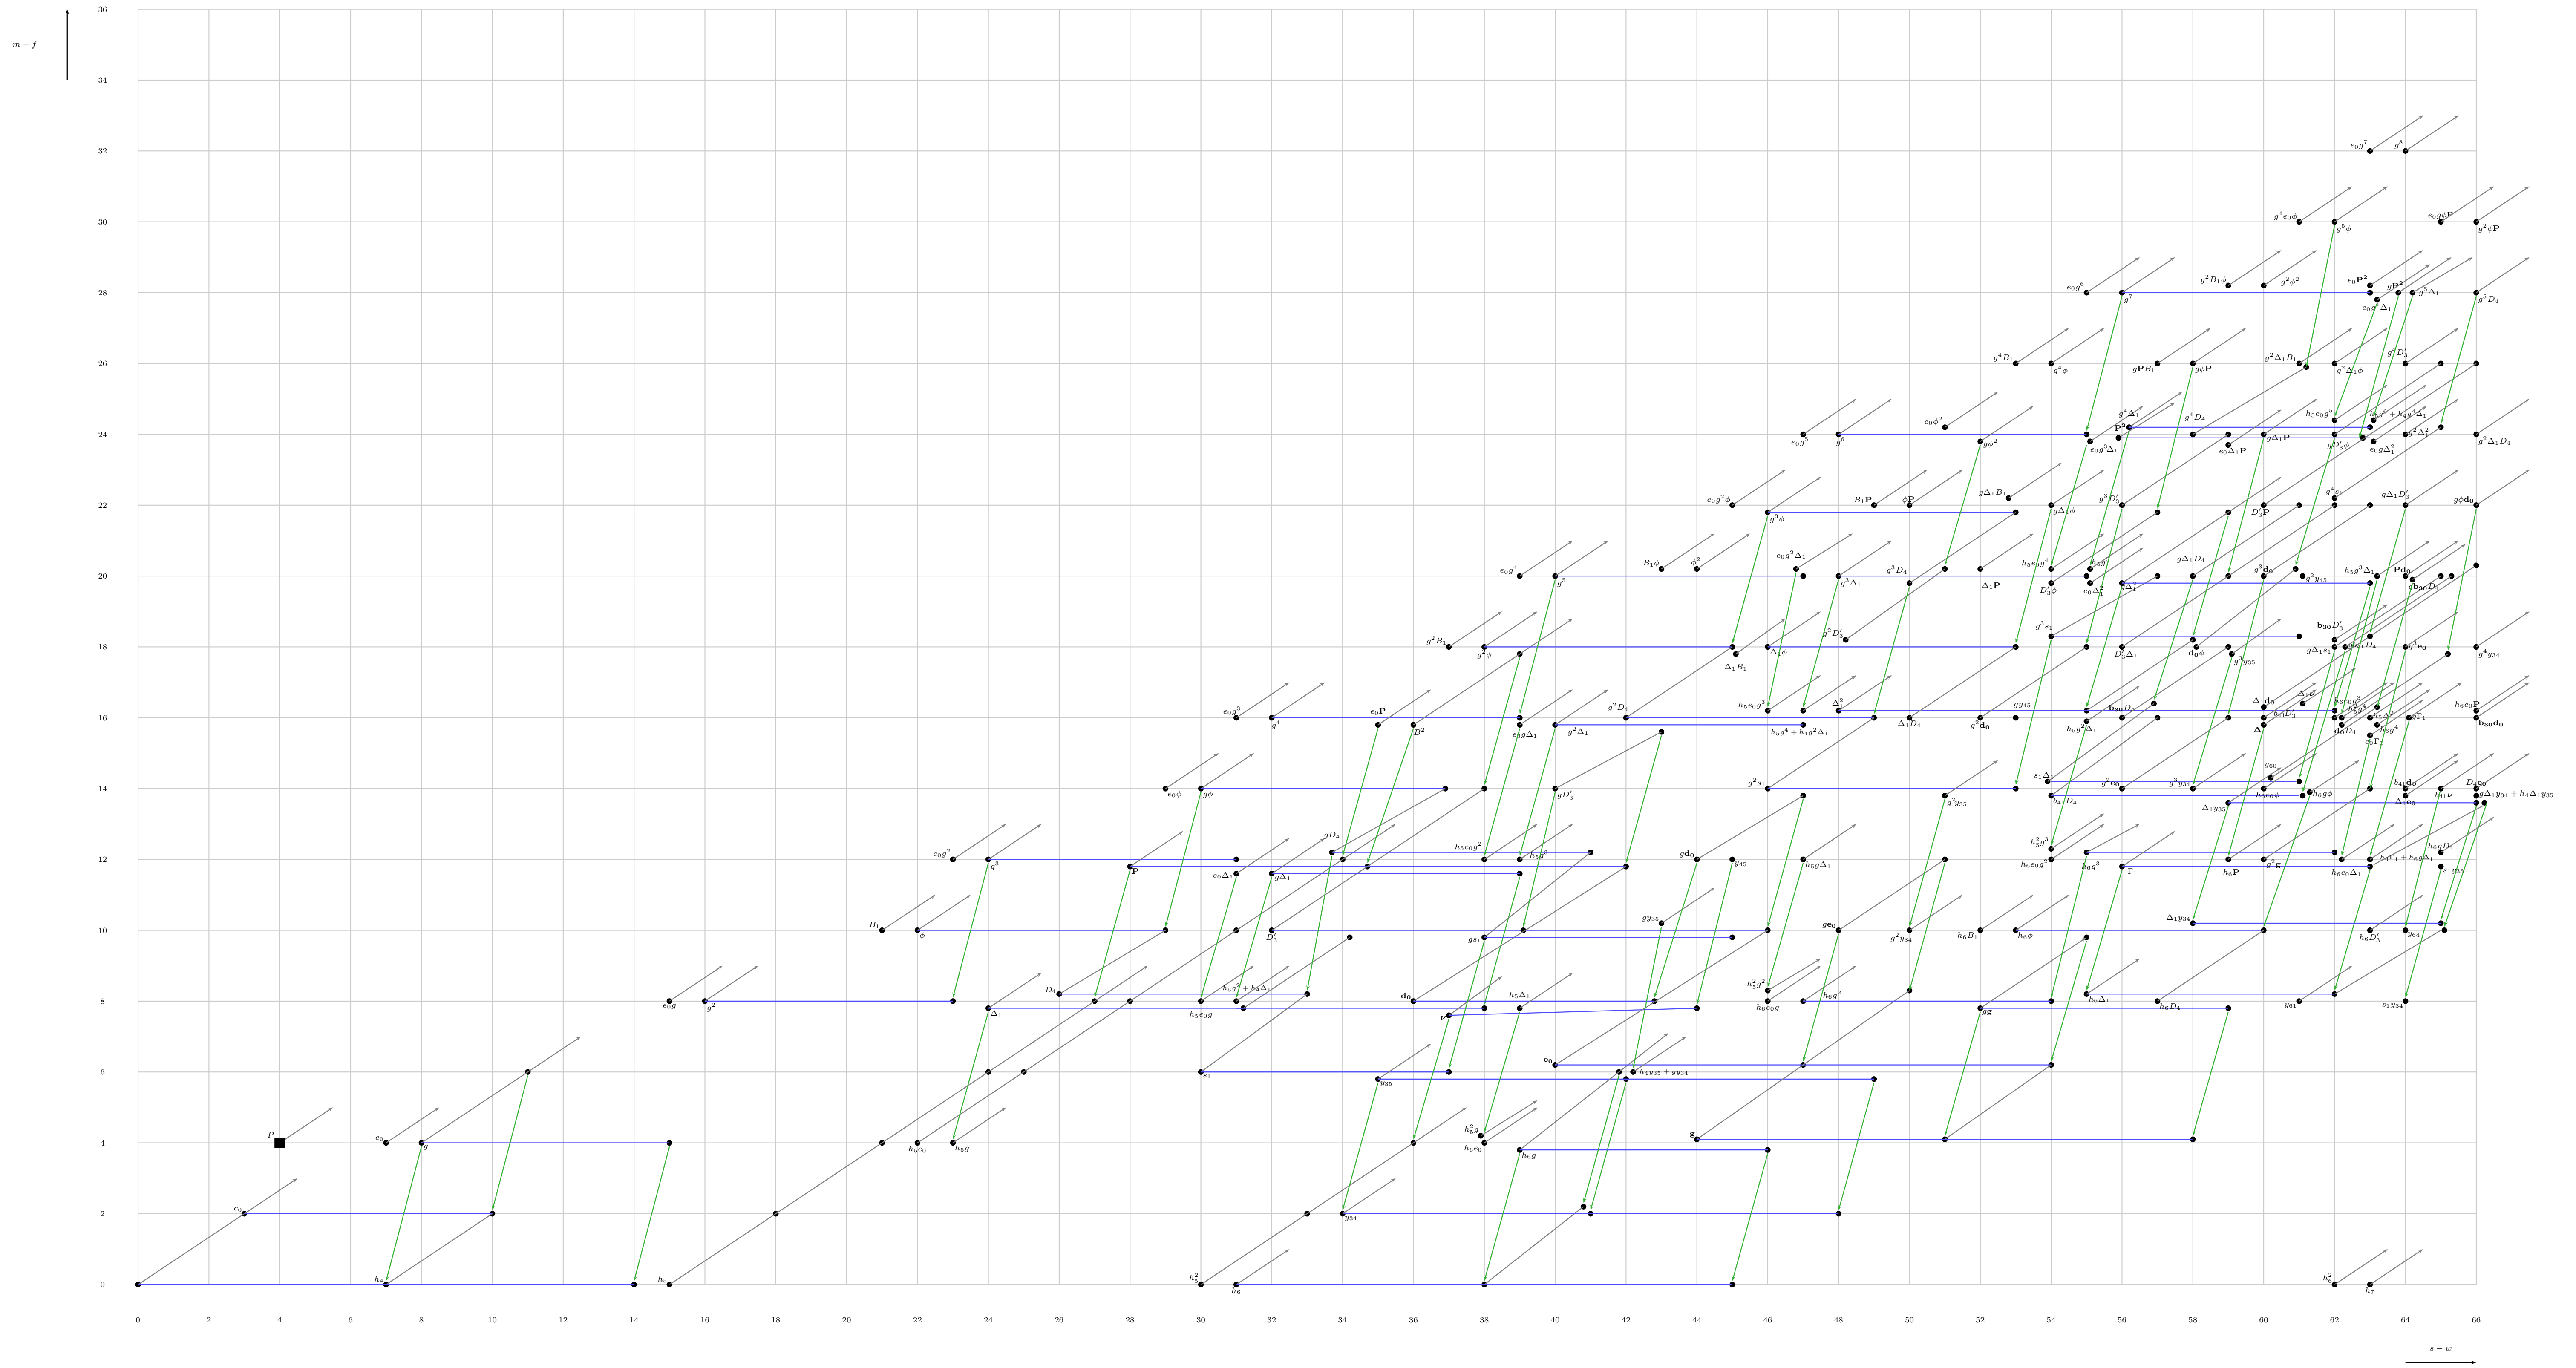

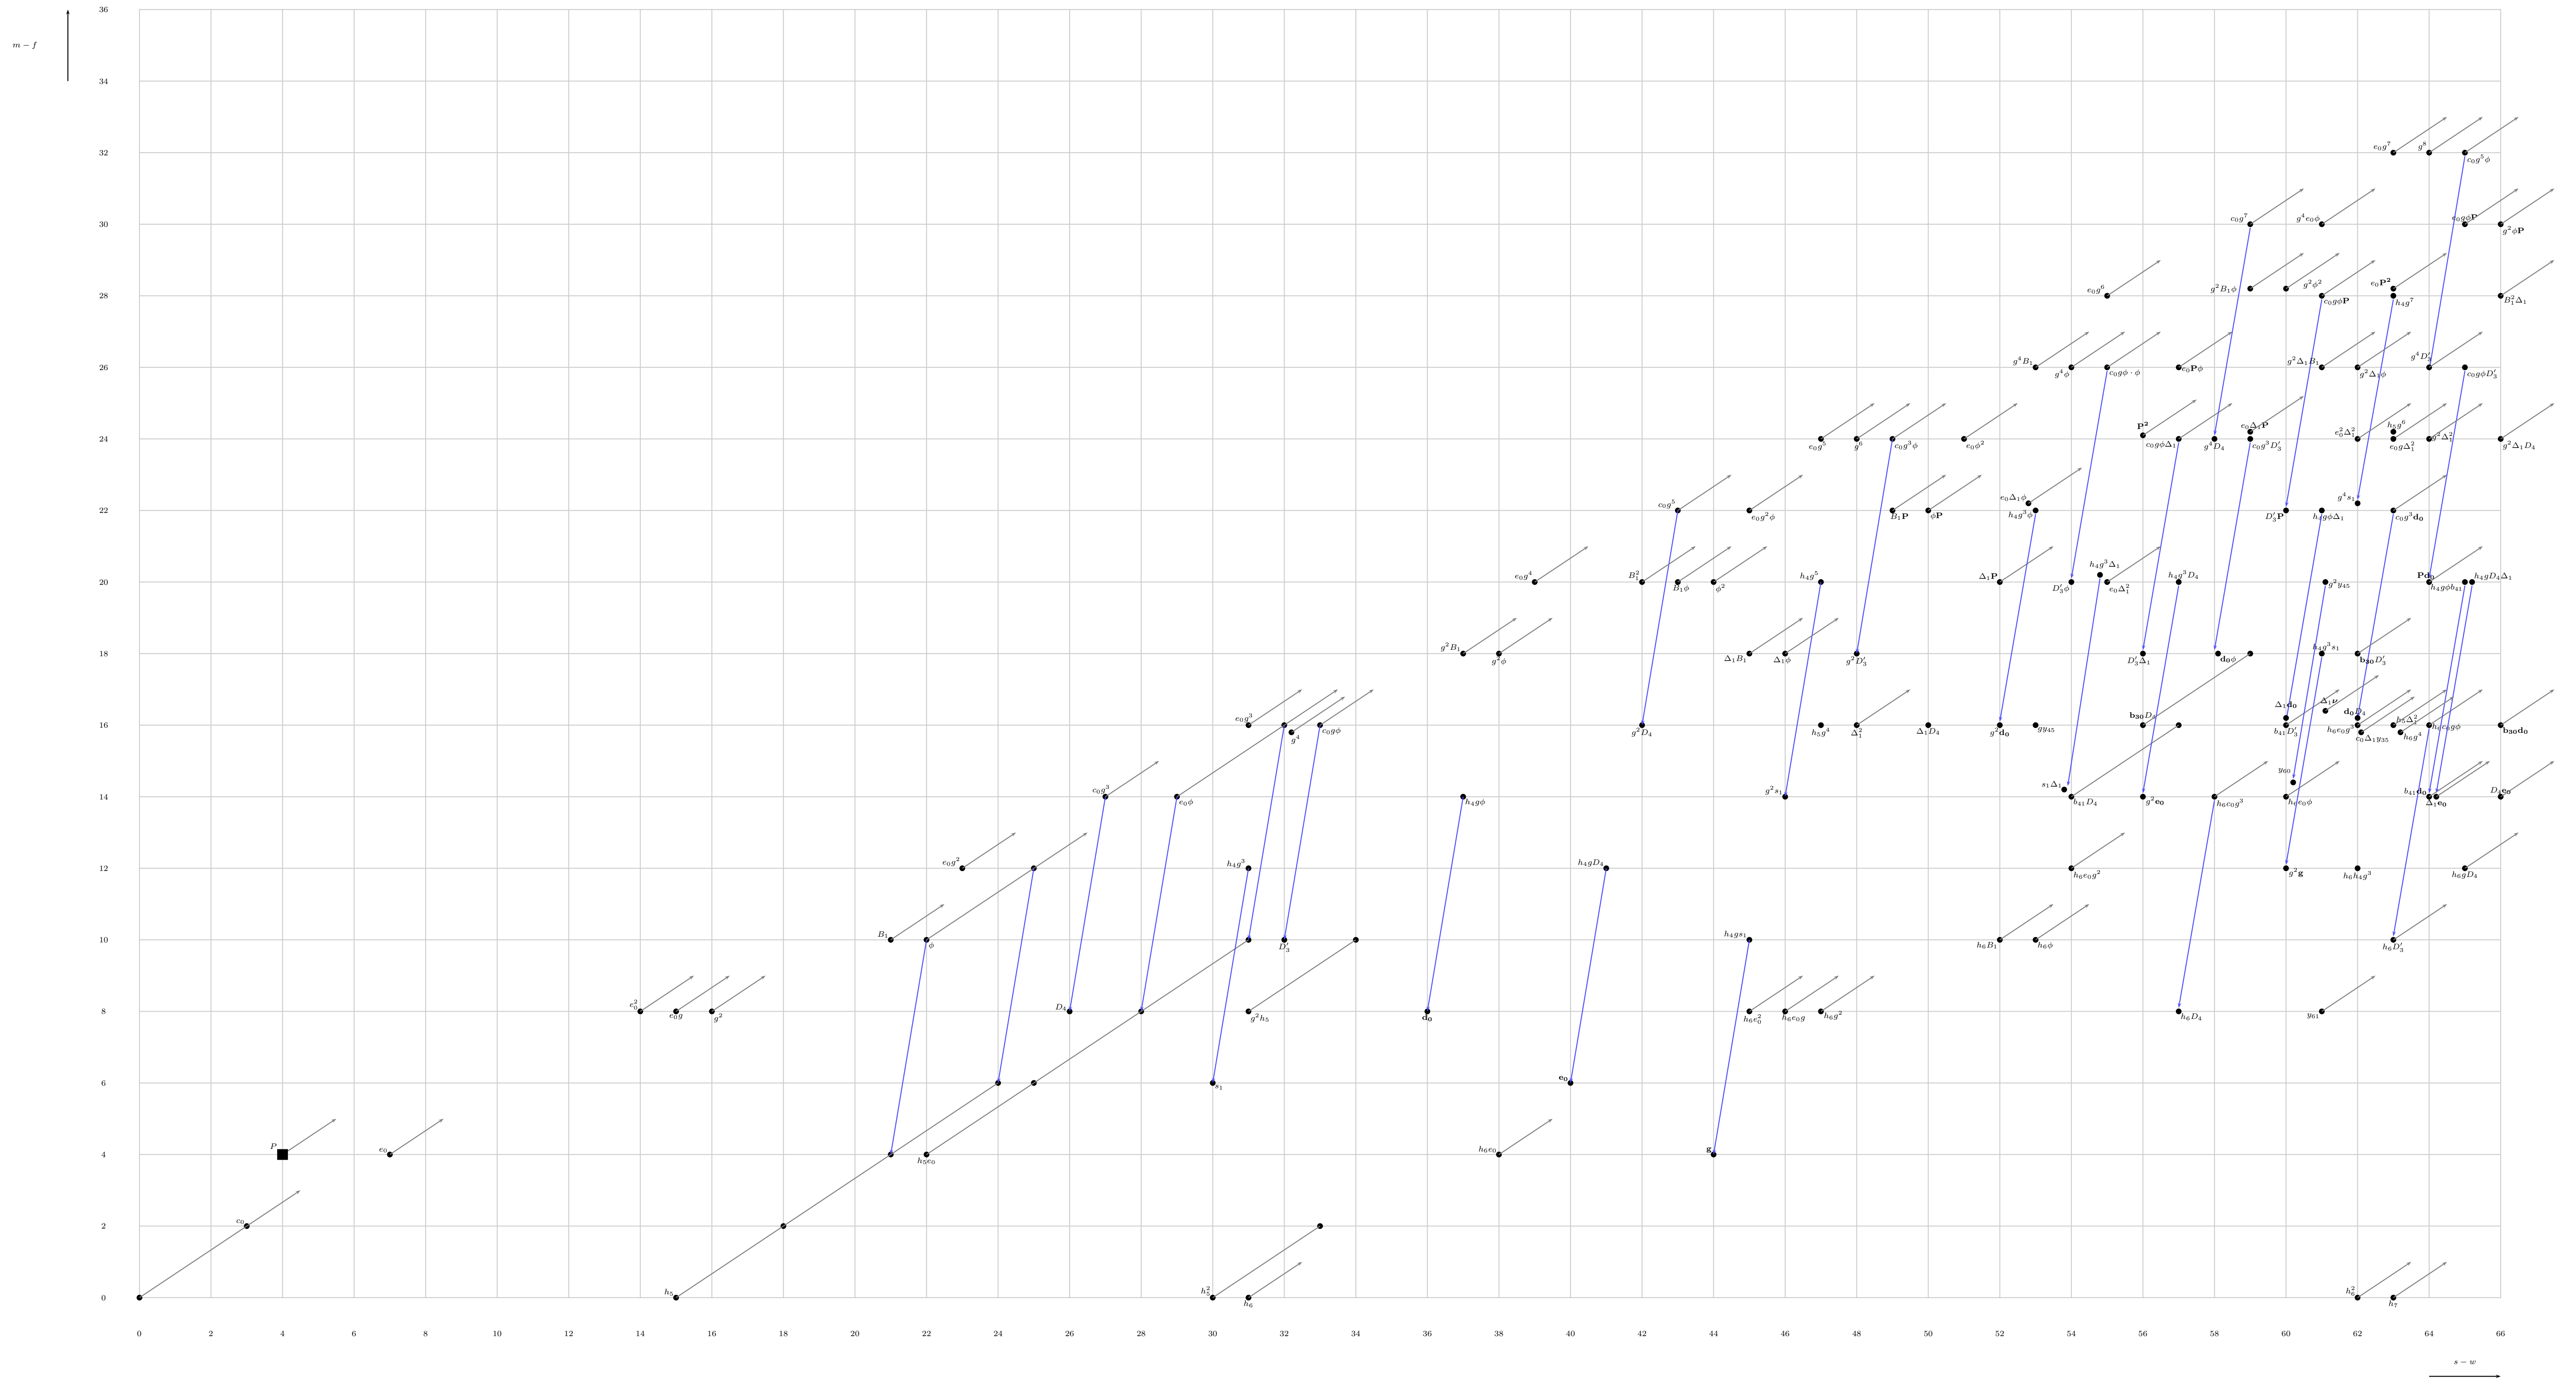



$E_{10}$ -PAGE OF THE  $h_1$ -LOCALIZED MOTIVIC MAY SPECTRAL SEQUENCE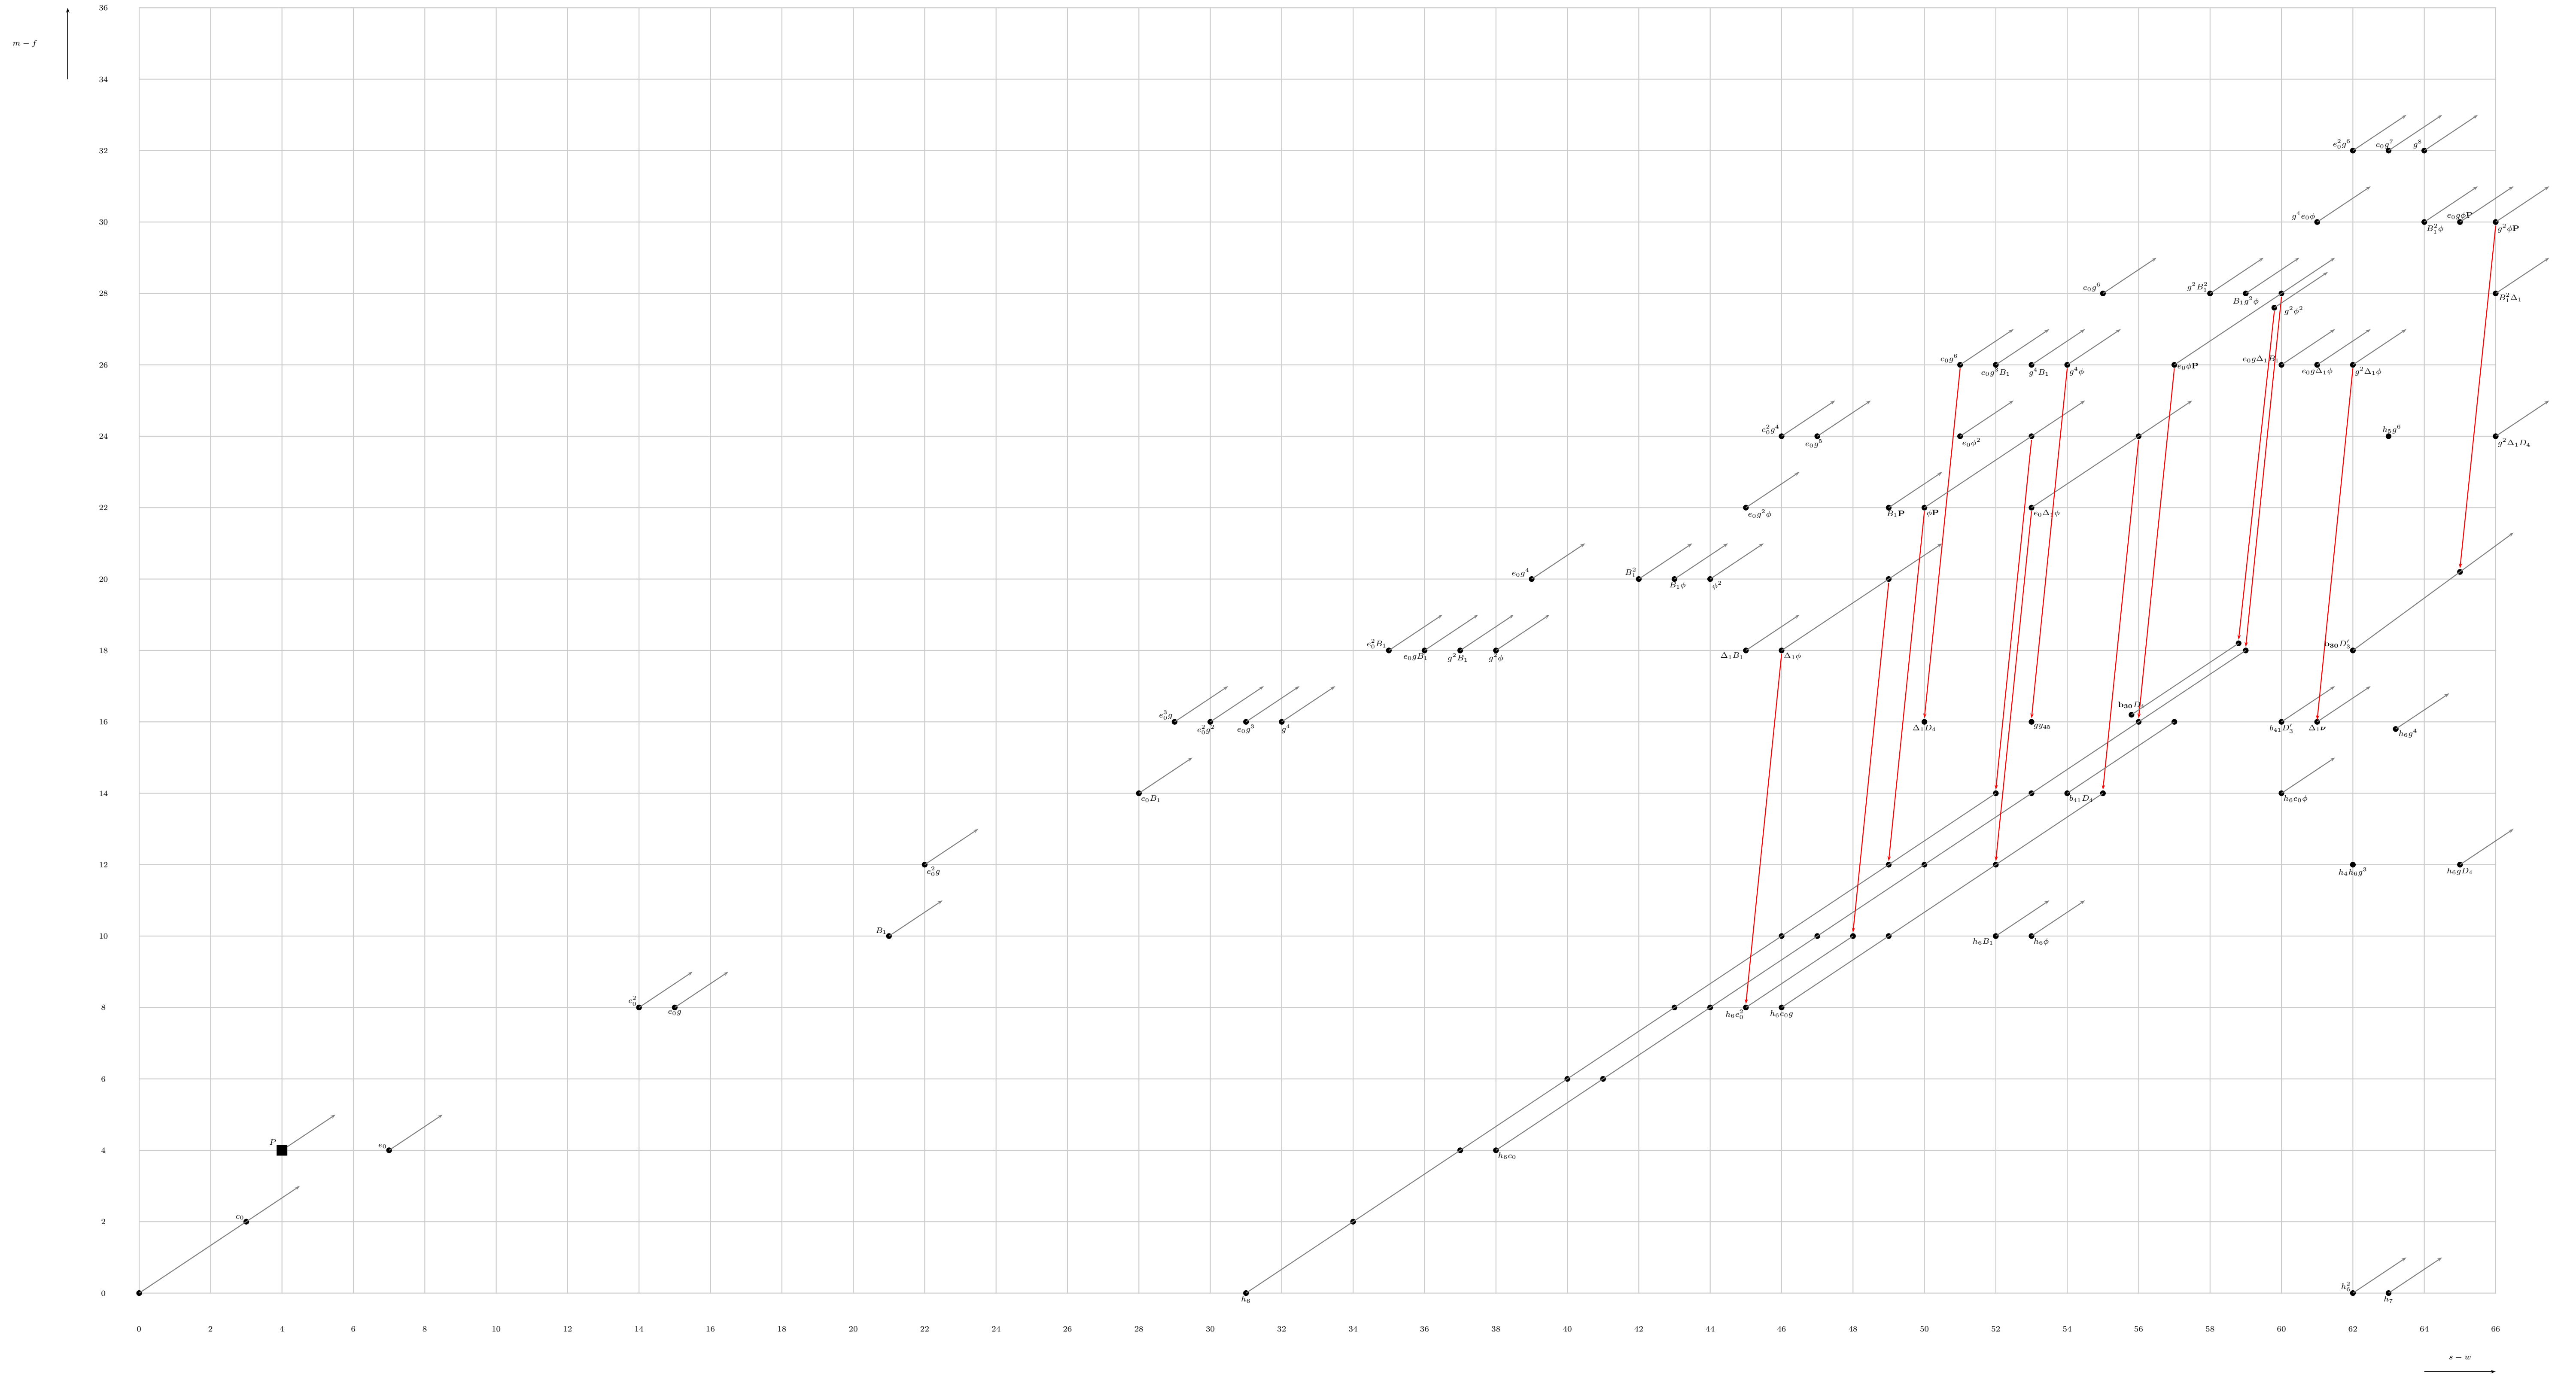







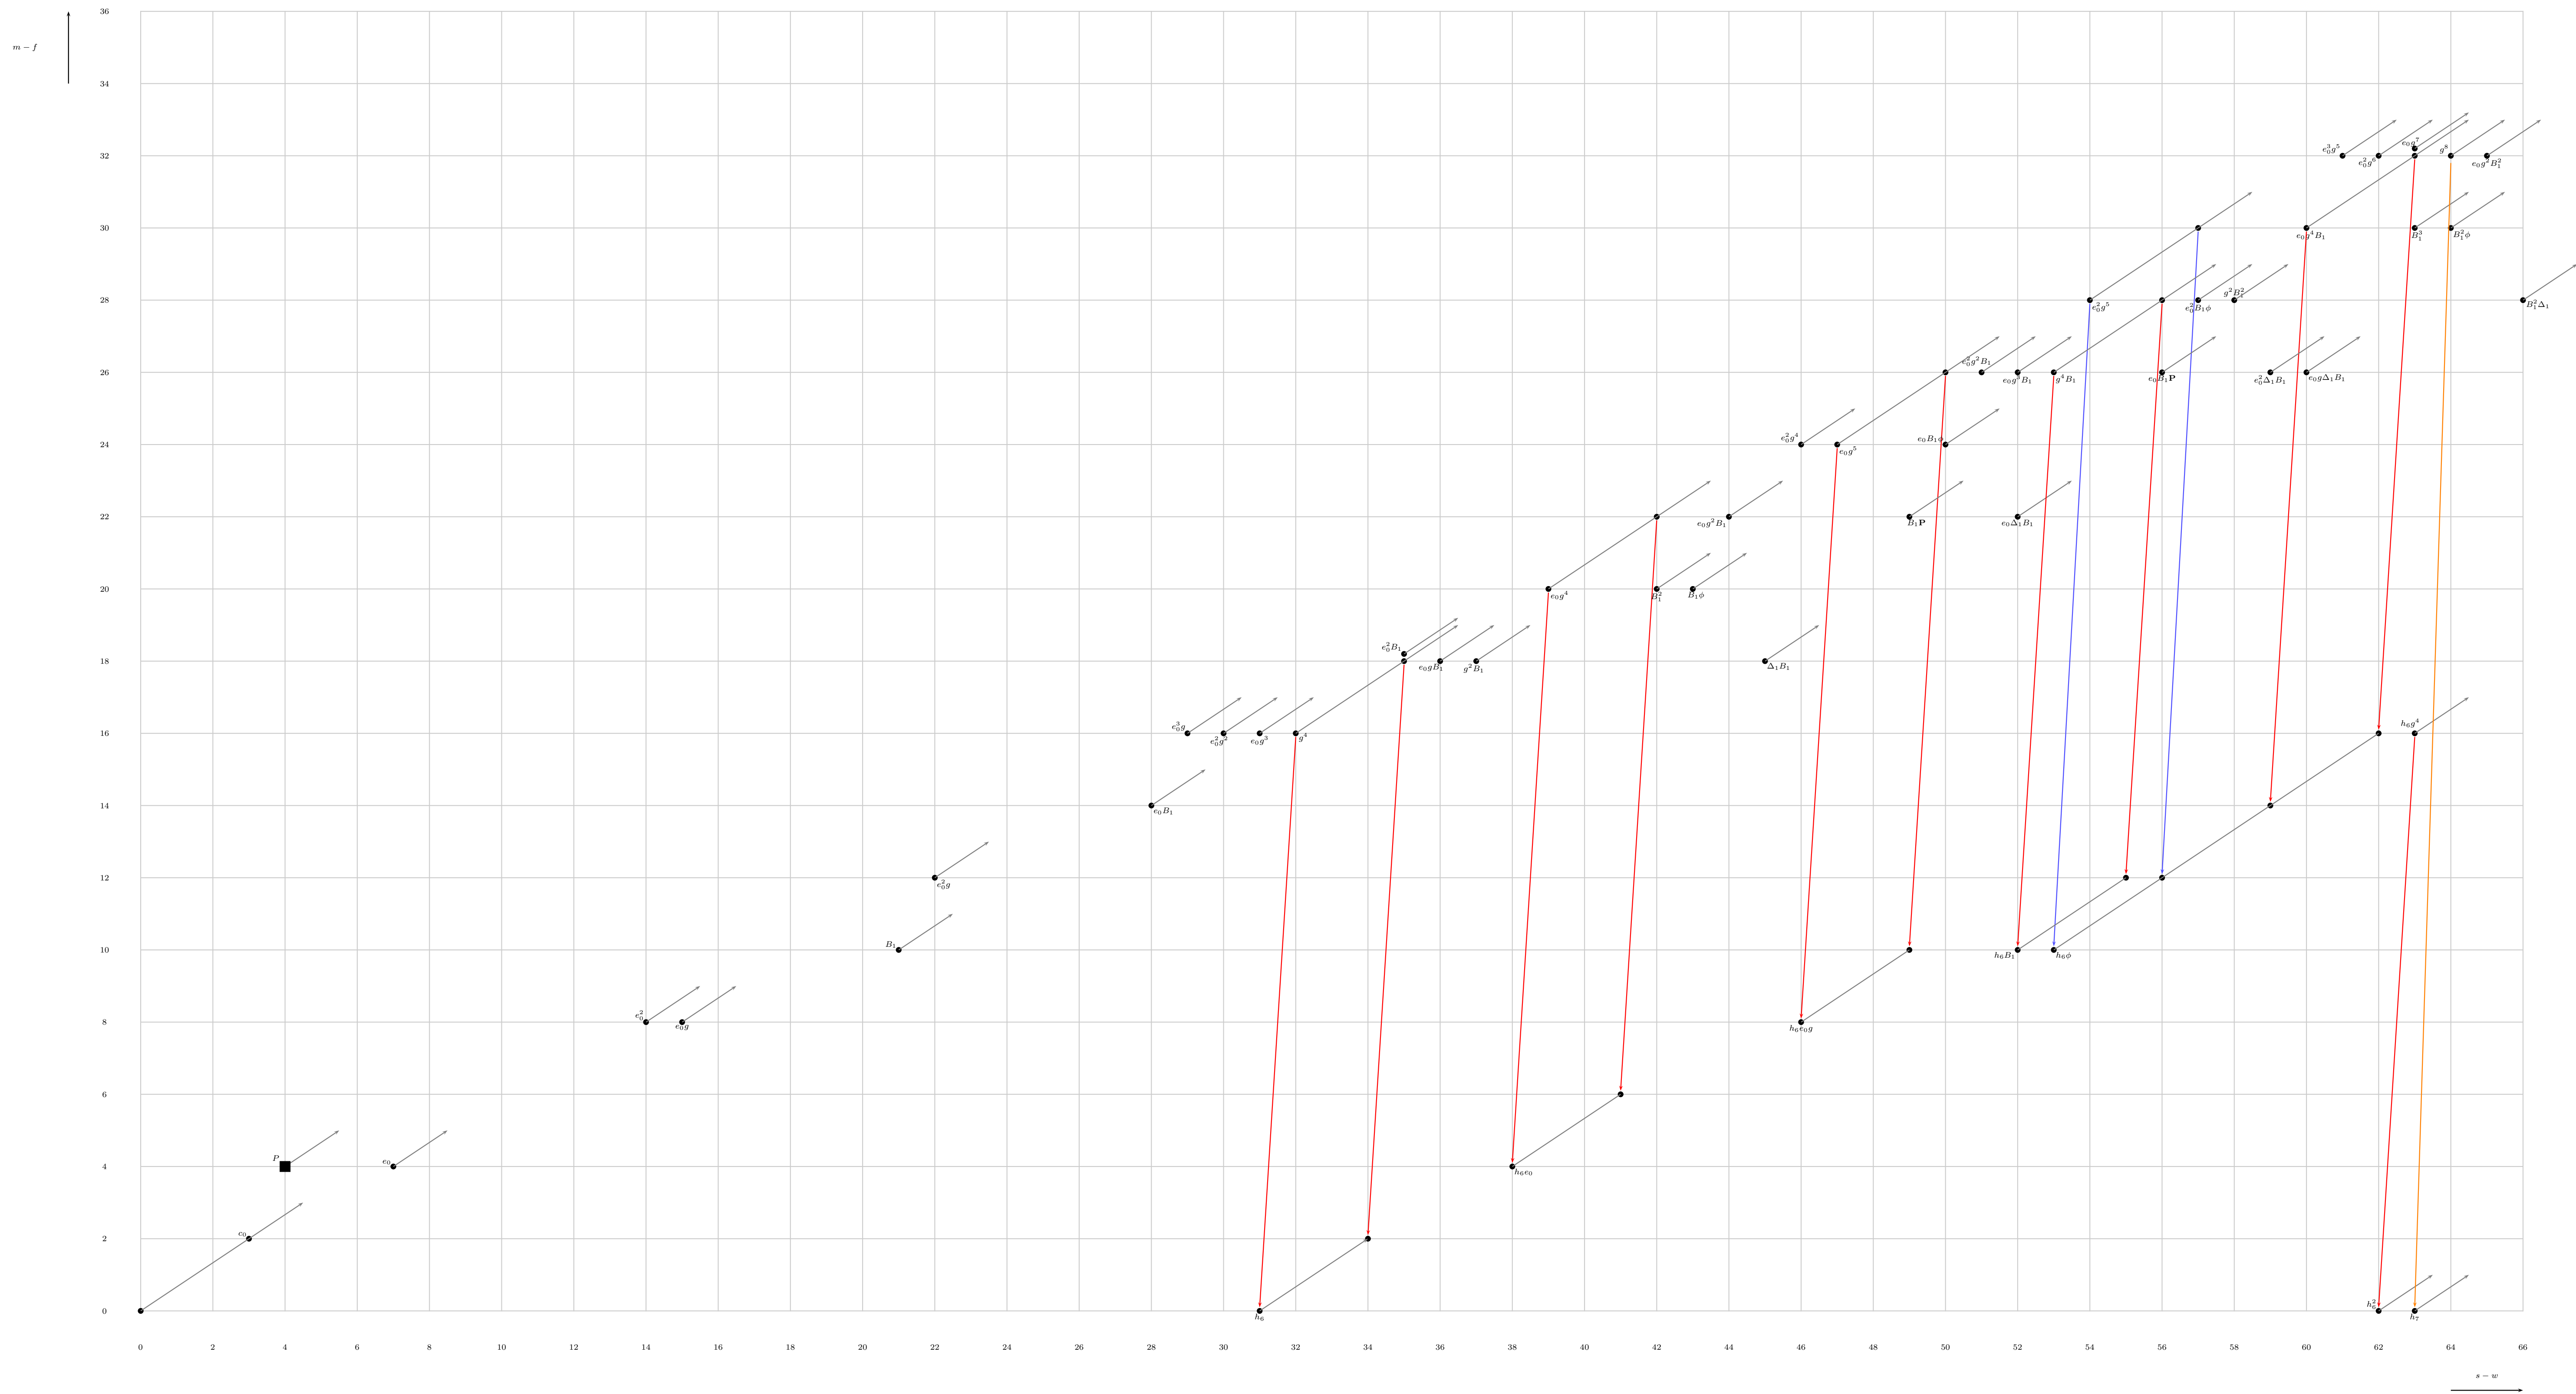



$E_\infty$ -PAGE OF THE  $h_1$ -LOCALIZED MOTIVIC MAY SPECTRAL SEQUENCE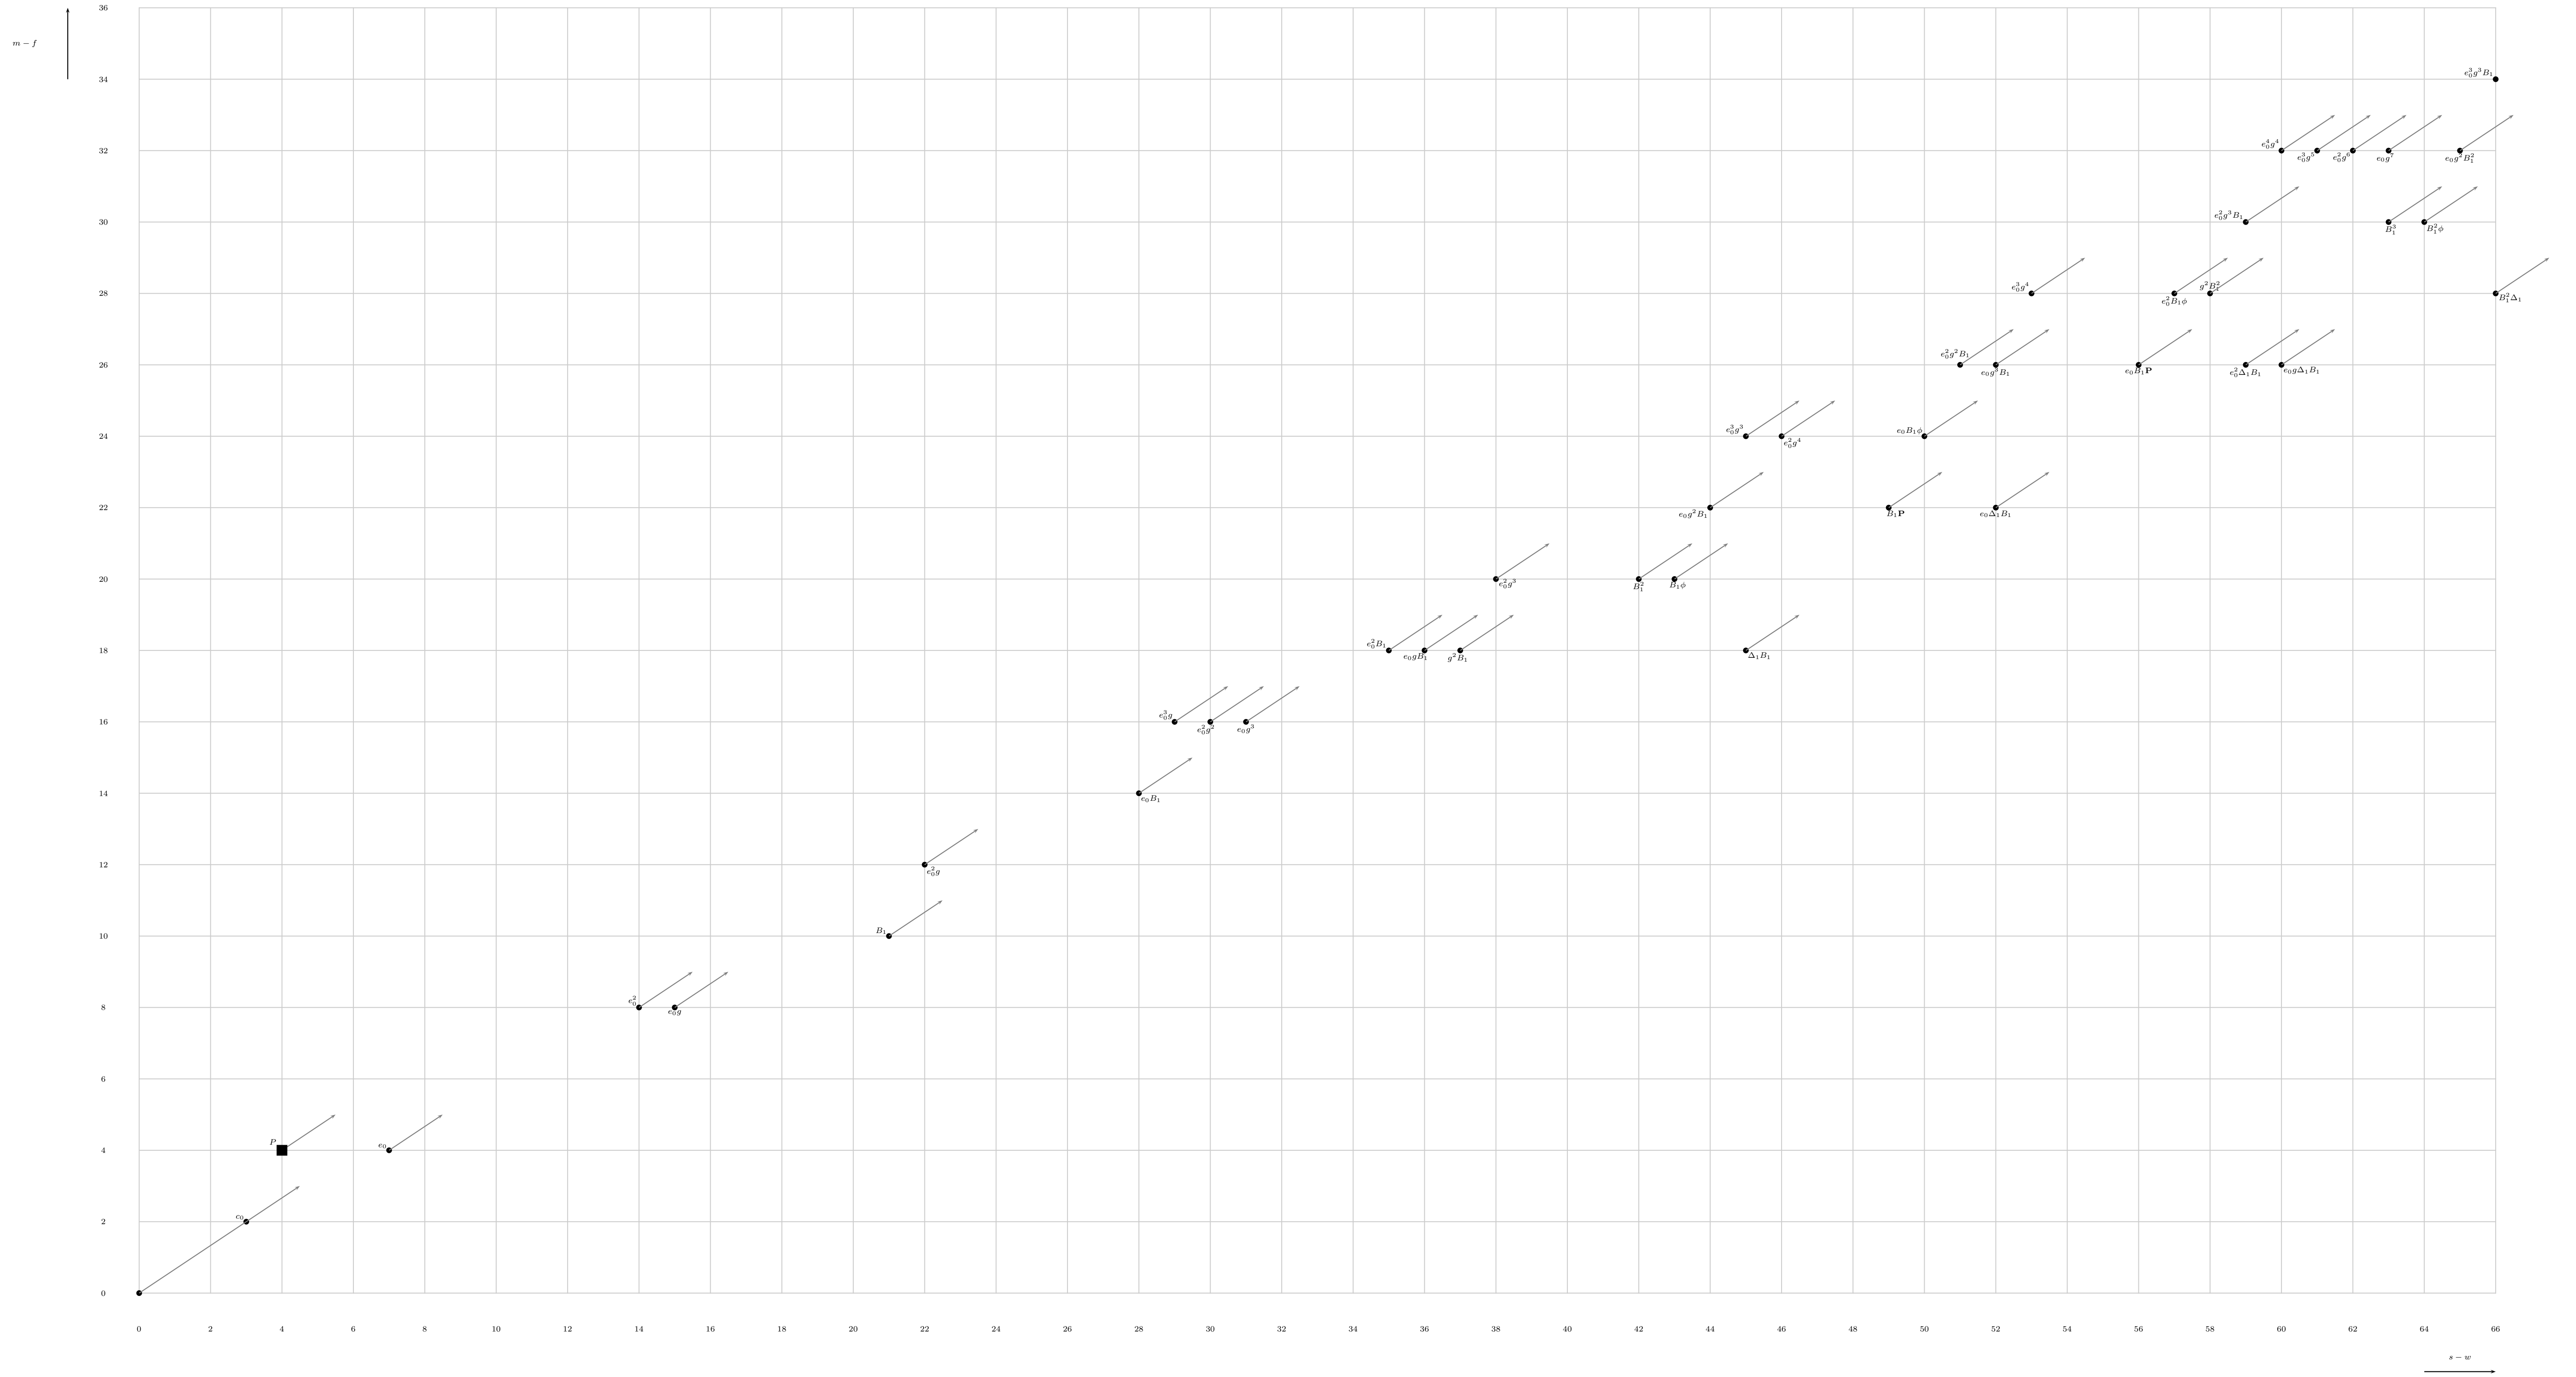

Supplement: Supplementary file 1 [file MayCharts.pdf]
